# Supplementary material for: {\alpha}Depth: Learning Scene-Level Soft Boundary Decomposition for Stereo Conversion
Source: arXiv:2606.00386 source file (2026-11-04)
Supplement: Supplementary file 1 [file fig-supp-limitation.tex]

% figs/supp/fig-supp-stability.tex
% Template: 2 rows x 6 columns (replace image paths accordingly)

\begin{figure}[t]
  \centering
  \begin{subfigure}[b]{0.33\textwidth}
    \centering
    \includegraphics[width=\linewidth]{imgs/supp/limitation/thor_145700/image.png}
  \end{subfigure}\hfill
  \begin{subfigure}[b]{0.33\textwidth}
    \centering
    \includegraphics[width=\linewidth]{imgs/supp/limitation/thor_145700/depth.png}
  \end{subfigure}\hfill
  \begin{subfigure}[b]{0.33\textwidth}
    \centering
    \includegraphics[width=\linewidth]{imgs/supp/limitation/thor_145700/alpha.png}
  \end{subfigure}
  % -------- Row 10 (with centered \caption* under each image) --------
  \begin{subfigure}[b]{0.33\textwidth}
    \centering
    \includegraphics[width=\linewidth]{imgs/supp/limitation/thor_78470/image.png}
    \caption*{Input Image}
  \end{subfigure}\hfill
  \begin{subfigure}[b]{0.33\textwidth}
    \centering
    \includegraphics[width=\linewidth]{imgs/supp/limitation/thor_78470/depth.png}
    \caption*{Input Depth}
  \end{subfigure}\hfill
  \begin{subfigure}[b]{0.33\textwidth}
    \centering
    \includegraphics[width=\linewidth]{imgs/supp/limitation/thor_78470/alpha.png}
    \caption*{Alpha Result}
  \end{subfigure}
  \caption{\textbf{Visual examples of failure cases}. Since \myname\ is designed based on the physical compositing model Eq.~(\ref{eq:alpha_composition}), it can fail in cases that violate the local two-layer model, \eg, volumetric media and glass/reflections.}
  \label{fig:supp-limitation}
  % \vspace{-em}
\end{figure}
